# Supplementary material for: Formation of Quantum Phase Slip Pairs in Superconducting Nanowires
Source: arXiv:1406.5128 source file (2015-05-27)
Supplement: Supplementary file 1 [file SOM.pdf]

# Supplemental Material for
# Formation of Quantum Phase Slip Pairs in Superconducting Nanowires

A. Belkin,[1] M. Belkin,[1] V. Vakaryuk,[2,3] S. Khlebnikov,[4] and A. Bezryadin[1,*]

[1]*Department of Physics, University of Illinois at Urbana-Champaign, Urbana IL 61801*

[2]*Department of Physics and Astronomy, Johns Hopkins University, Baltimore, MD 21218*

[3]*American Physical Society, 1 Research Road, Ridge, NY 11961*

[4]*Department of Physics and Astronomy, Purdue University, West Lafayette, IN 47907*

(Dated: March 27, 2015)

* bezryadi@illinois.edu

### 1. Molecular templating

Molecular templating [1] allows us to make nanowires with small diameters, which are seamlessly connected to external thin film electrodes. The measurements on such nanowires are not jeopardized by the unwanted contact resistance between the nanowire and the electrodes. The technique works as follows. A trench with an undercut is made on a Si substrate covered with a film of $SiO_2$ and a low stress $Si_3N_4$ film. Fluorinated carbon nanotube are deposited over the substrate with the trench (see Fig. S1) from a solution in isopropanol. Some tubes fall across the trench. The top surface is then sputter-coated with a superconducting alloy, amorphous $Mo_{76}Ge_{24}$. The nanotubes crossing the trench thus become superconducting nanowires (SNW) because their outer surface becomes decorated with the superconducting alloy. Both the film and the nanowires are formed during the same sputtering session, allowing to avoid any contact resistance. The resonator is then shaped using standard photolithography and wet etching in hydrogen peroxide. The photo mask is positioned such that only two nanowires are protected by the photoresist. The etching process not only shapes the resonator but also ensures the destruction of all nanowires except the selected pair, which is protected by the photoresist.

Sample B has the following parameters: nanowires' length is 200 nm, nanowire width is 25-30 nm, and thickness is 20 nm. The distance between the nanowires is $w_{wire} = 10\,\mu$m. The distance between the input and output "mirrors" of the Fabry-Perot coplanar waveguide resonator for both samples is 6 mm. The resonance frequency of the fundamental mode for sample B is $f_0 \sim 5.5$ GHz. The width of the center conductor of the resonator is $w_{cc} = 20\,\mu$m. The input, output and the ground planes are partially covered by 100 nm thick gold film (Fig. 1) to facilitate the connection of external gold wires to them. Standard gold wires, in ultrasonic wire bonder, have been used to connect the input and the output ports of the resonator to external microwave measurement lines. Gold wires have been chosen because they stay normal at sub-Kelvin temperatures and allow a good thermal anchoring of the sample to the Faraday cage. We chose not to use aluminum wires, which are frequently used in wire bonders, because Al becomes superconducting and thus might cause Meissner loops and might have a low thermal conductivity at sub-Kelvin temperatures, thus preventing good thermalization of our coplanar waveguide resonator with nanowires.

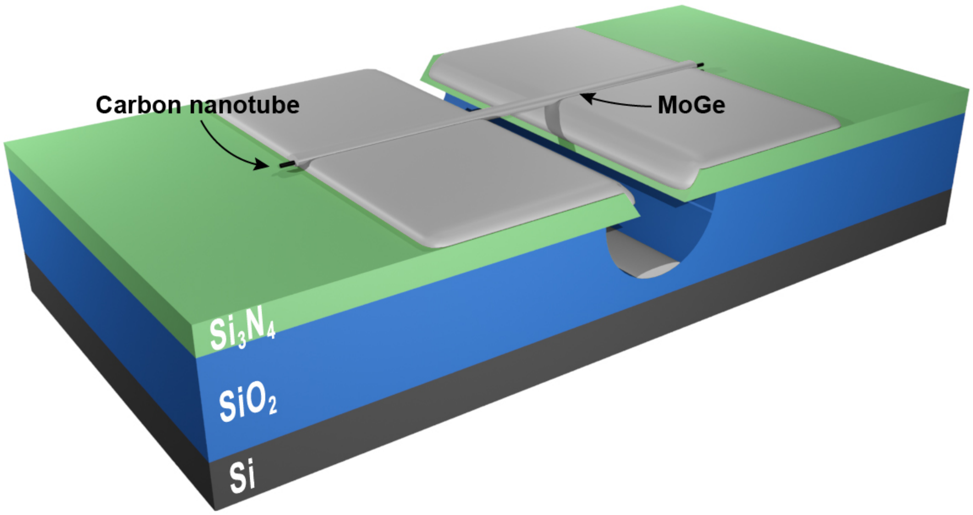


Fig. S 1. Schematic view of the molecular templating technique. Fluorinated carbon nanotube is stretched across a trench etched into $Si_3N_4/SiO_2$ on a Si chip. The nanotube and the banks are coated with superconducting $Mo_{76}Ge_{24}$. The coplanar waveguide resonator is not shown in this schematic drawing.

## 2. Low-temperature setup: $^3$He and dilution refrigerator

To study the rates of phase slips in nanowire loops as a function of magnetic field we employed two different cryogenic systems, *i.e.* $^3$He and a dilution refrigerator. Below we describe the microwave input and output lines for both of them.

**$^3$He microwave input line:** Input SMA connector to 4 K stage – stainless steel semirigid cable providing ∼-11 dB attenuation at 5 GHz, -20 dB attenuator at 4 K stage, -3 dB attenuator at 1 K pot stage, -13 dB attenuator at 0.3 K stage. The attenuators have been used to thermalize the microwave signal line. The lowest-temperature attenuator was connected through a copper cable to the Faraday cage in which the sample was installed.

**$^3$He microwave output line:** Sample Faraday cage ⇒ -18 dB isolator at 0.3 K stage ⇒ -18 dB isolator at 1 K pot stage ⇒ +40 dB low temperature amplifier (Low Noise Factory, LNF-LNC4_8A) at 4 K stage ⇒ stainless steel semirigid cable with ∼-11 dB of attenuation ⇒ output SMA connector on top of the cryostat.

**Dilution fridge microwave input line:** The input SMA connector was connected to the 4 K stage through a stainless steel semirigid cable providing ∼-11 dB attenuation at 5 GHz. Then the circuit includes -10 dB attenuator at 4 K stage, -10 dB attenuator at 1 K pot

stage, -3 dB attenuator at heat exchange stage, -20 dB attenuator at mixing chamber stage. The lowest temperature attenuator is connected to the Faraday cage with the sample by means of a Cu coaxial cable.

**Dilution fridge microwave output line:** Sample Faraday cage ⇒ -20 dB isolator at mixing chamber stage ⇒ -20 dB isolator at heat exchange stage ⇒ +32 dB low temperature amplifier (Low Noise Factory, LNF-LNC6_20A) at 1 K pot stage ⇒ -3 dB attenuator at 4 K stage ⇒ stainless steel semirigid cable with ∼-11 dB of attenuation ⇒ output SMA connector.

### 3. Phase slip distributions for sample B

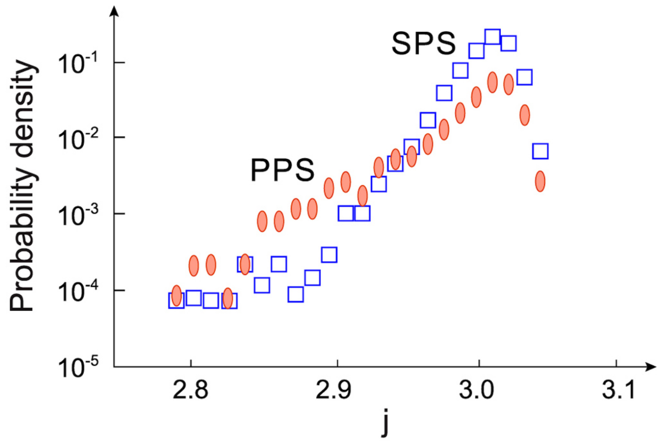


Fig. S 2. Probability densities of SPS and PPS as functions of normalized current in solenoid. Blue squares correspond to SPS, red – to PPS transitions. Data is obtained from sample B, measured at $T = 350\,\mathrm{mK}$.

The rates of SPS and PPS, detected in sample B, are plotted in Fig. S2 as functions of the current in the solenoid normalized by the corresponding Little-Parks period. As one can clearly see, probability density curves intersect. This results confirms the dominance of QPPS in the low current regime. The apparent noise level is about $2{\cdot}10^{-4}$. This higher noise level, compared to sample A, is due to the higher bath temperature (sample A – 60 mK, sample B – 350 mK) and lower numbers of measurements included in the statistical analysis of the probability distributions and the rates.

### 4. Critical temperature of superconducting nanowires and the quantum-classical crossover temperature

The critical temperature of MoGe nanowires can be estimated based on the wire cross sectional area, $S$. Using the dependence from S-Ref. [2], we find $T_c \approx 5.3\,\mathrm{K}$ for $S \approx 400\,\mathrm{nm}^2$ (sample A). Once the critical temperature is obtained, the expected crossover temperature $T_q$ is readily calculated from the linear relationship S-Ref. [1] ($T_q = 0.164\,T_c$), giving us $T_q = 0.87$ K. Note that such estimate is similar in value to the experimentally observed crossover temperature $T_q$.

### 5. Calculation of phase slip probability density, standard deviation and rate

We calculate phase slip probability density, standard deviation and rate using the following formulas:

$$P_x(j) = \frac{n_x(j)}{n(j)}$$

$$\sigma_x(j) = \Big(\frac{1}{N_x - 1}\sum_{i=1}^{N_x}(j_{x,i} - \bar{j_x})^2\Big)^{1/2}$$

$$\mathit{\Gamma}_x(j) = \frac{v_J}{\Delta j}\cdot\frac{n_x(j)}{N_T(j)}$$

Here $n_x(j)$ is a number of phase slips of type $x$ ($x \rightarrow SPS$ or $PPS$) observed in the current interval $\Delta j$ centered at $j$, $n(j)$ is the number of all phase slips in the same current interval, $N_x$ is the total number of phase slips of type $x$ in the distribution, $j_{x,i}$ is $i^{th}$ switching current of type $x$, $\bar{j_x}$ is the average switching current of type $x$, calculated as $\bar{j_x} = \frac{1}{N_x}\sum_{i=1}^{N_x} j_{x,i}$, $N_T$ is the total number of phase slips observed at currents greater than $j$.

### 6. Influence of external photons on PPS probability

To verify that PPS are not caused by a stray electromagnetic radiation from the environment, we covered the inner part of the Faraday cage by radiation-absorbing black coating S-Ref. [3] that has an absorptivity of 90 % over a wide angle in the 0.3 - 2.5 THz range S-Ref. [4]. In addition, we reduced the input power sent to the resonator by 5 dBm. The impact of these two modifications on the probability of PPS is shown in Fig. S3. There, we plot the difference between probability densities of PPS and SPS events, ($P_{PPS}-P_{SPS}$), as a function of normalized current $j$ before and after the above changes have been made. (We

remind here that the normalized current is obtained by dividing the current in the solenoid by the Little-Parks oscillation period, also expressed in terms of the current in the solenoid.)

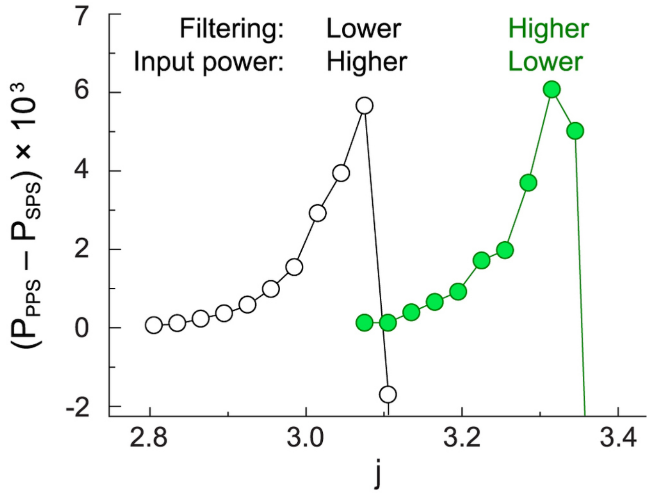


Fig. S 3. Comparison of different measurement conditions. Difference between PPS and SPS probability densities before (black circles) and after (green circles) the infrared absorbing coating is added and the input power is reduced.

It is clear that the peak height, describing the predominance of PPS over SPS, has not become smaller after we reduced the probe microwave power and added the black coating absorbing background noise photons. We also find that in the case of better filtering, the net percentage of PPS increased from 18 % to 34 %. These facts make us confident that the observed much higher rate of PPS (at sufficiently low bias magnetic field) is not induced by external perturbations. On the contrary, it appears as a delicate macroscopic quantum phenomenon, which is weakened by the slightest external perturbation, such as not perfect filtering of the external noise or a slightly increased measurement signal power. In conclusion, we find that the relative rate of PPS, if compared to SPS, is higher in electromagnetically "quieter" environments.

**7. Expected values of $\alpha$ and $C_2$**

Our quantitative estimate of the QPPS rate is based on the Korshunov's instanton solution [5]. We encapsulate the difference between a Josephson junction, for which the instanton was originally found, and a nanowire by taking the instanton-antiinstanton interaction to be of the same (dipole) form as in S-Ref. [5], but with a magnitude proportional to a free

parameter $\alpha$ (a constant of order unity). In S-Ref. [5], $\alpha$ is approximately 2, while in our case a good fit to the data is achieved with $\alpha = 6$. This difference is probably due to the fact that the spatio-temporal form of the phase slip in thin wire does not coincide exactly with the form of the phase slip in a Josephson junction, for which Korshunov's theory was developed.

The effective capacitance for the paired phase slips, $C_2$, is not related to the capacitance of the waveguide. This is because the two phase slips entering the loop, one through each wire, move in opposite directions. Therefore, they create opposite charges on the electrodes, which compensate each other. So, charging of the electrodes does not happen and consequently the capacitance of the electrodes is not relevant. Therefore, the relevant capacitance, which determines the effect of inertia in paired phase slip events, can roughly be estimated as the self-capacitance of the nanowires. To estimate this capacitance $C_2$, we use the expression for a cylindrical capacitor: $C = 2\pi\epsilon\epsilon_0 L_c/\ ln(R_{out}/R_{in})$. Here $\epsilon$ is the dielectric constant, $\epsilon_0$ is the vacuum permittivity, $L_c$ is the length of the capacitor, $R_{out}$ and $R_{in}$ are the outer and inner radii of the capacitor, respectively. Applying this formula to our system we associate $L_c$ with the nanowire length, which is about 200 nm, $R_{in}$ – with its radius ($\sim$10 nm), and $R_{out}$ – with the distance to an effective ground. The latter quantity could be estimated as the distance from the nanowire center to the c.c. strips, *i.e.* as $L_c/2$ ($\sim$100 nm). If the dielectric constant $\epsilon = 1$, we obtain $C_2 \approx 0.5 \times 10^{-17}$ F.

## 8. Analysis of SPS and PPS rates for sample B

From the distributions presented in Fig. S2 we calculate the corresponding rates of SPS and PPS for sample B. The results (see Fig. S4) demonstrate that $\Gamma_{SPS}$ and $\Gamma_{PPS}$ have qualitatively the same behavior as for sample A, although the noise floor is somewhat higher (of the order of 0.02 switching events per second).

We were able to fit the rate of SPS using the following parameters: $\Omega = 2.3 \cdot 10^{11}$ Hz, $I_c = 8.0\,\mu$A, $j_c = 3.51$. From the best fit for the QPPS rate we find that $A_2 = 93.6$, $B_2 = 7.3 \cdot 10^{-37}$ 1/s, $j_c = 3.51$. These fitting parameters are close to those obtained for sample A.

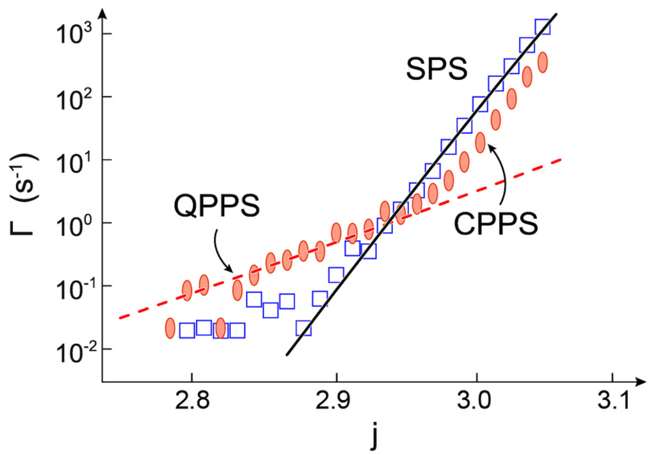


Fig. S 4. Rates of SPS and PPS as functions of normalized current in the solenoid for sample B. The bath temperature is 350 mK. Single (blue squares) and paired (red ovals) phase slip rates are obtained from the distributions shown in Fig. S2. The solid black line is the Kurkijärvi-Garg fit for SPS, the dashed red line is the Korshunov fit for QPPS.

### 9. Guinea-Schön-Korshunov action for SPS and QPPS

Our starting point is the Euclidean action for a Josephson junction in the case when a dissipative component with the single-electron charge periodicity is present (see Eq.1). In the case of paired phase slips, assuming that one phase slip occurs on each wire, the Caldeira-Leggett dissipation, *i.e.* the quantum dissipation, is associated with a closed-circle motion of unpaired electrons or Bogoliubov quasiparticles in the loop formed by the nanowires. The origin of these single-electron-type excitations is not well understood. These gapless or approximately gapless quasiparticles might occur due to the oxidized, strongly disordered surface of the nanowire, or due to strong disorder accompanied by enhanced Coulomb interactions in mesoscopic nanowires, and brought about by the normal cores of the phase slips. This action we consider is given by the following equation S-Ref. [5–7]:

$$S[\phi\,(t)] = \int dt \left[\frac{m}{2}\left(\frac{\partial\phi}{\partial t}\right)^2 - \frac{I_c}{2e}\cos\phi - \frac{I}{2e}\phi\right] + \frac{4\eta}{\pi}\int\int dt dt' \frac{\sin^2\{[\phi\,(t) - \phi(t')]\,/4\}}{(t-t')^2} \quad (1)$$

The last term describes the influence of the quantum dissipation on the macroscopic quantum tunneling events (either SPS or QPPS).

Although we do not expect the cosine form of the potential and the sine form of the dissipative term to apply exactly to the case of nanowires, the semi-quantitative arguments of

this section are based on the periodicity properties, such as the $2\pi$ periodicity of the current-phase relationship (CPR) of the nanowires. Also, empirically speaking, superconducting nanowires can typically be described quite accurately by the equations derived for Josephson junctions, because both types of systems belong to the general class of superconducting weak links.

A tunneling event can be thought to occur around a certain value of the Euclidean time, when the phase $\phi(t)$ changes by $2\pi$ (for SPS) or $4\pi$ (QPPS). In the former case the last term in (1) logarithmically diverges at large values of $t - t'$, while in the latter case it remains finite [5]. As a result, at low temperatures and currents, tunneling by $2\pi$ is additionally suppressed. A qualitative explanation of this is as follows. When an SPS happens, the system tunnels from one minimum of the washboard potential to the next one, changing the phase of the condensate by $2\pi$. During this event, a small voltage develops and rotates the phase of the normal electrons, coupled to the condensate, by $\pi$ (assuming that normal electrons in the environment are quasi-independent and can be described by separate single-particle wave functions). Since the environment can be considered infinitely large for all practical purposes, such a change of the normal-electron phase is "too heavy" for the tunneling to occur. On the other hand, if the phase of the condensate rotates by $4\pi$, the corresponding rotation of the phase of the normal electrons is $2\pi$, which is a trivial change since the wave functions are $2\pi$-periodic. Therefore, cotunneling or tunneling by $4\pi$ in the washboard potential is not suppressed as strongly.

The same conclusion can be reached by analyzing Eq. 1. To make a simple estimate, let us assume that the phase slippage happens at $t = 0$ and that the phase changes instantaneously. Both for QPPS and SPS, $\phi(t) = \phi(t') = 0$ if $t < 0$ and $t' < 0$. Also, for $t > 0$ and $t' > 0$ the same is true: $\phi(t) = \phi(t') = 0$. Thus, the quantum dissipation (the last integral in Eq. 1) is zero both for $[t < 0\ ;\ t' < 0]$ and $[t > 0\ ;\ t' > 0]$ quadrants of the $t - t'$ plane. The situations in the quadrants $[t < 0\ ;\ t' > 0]$ and $[t > 0\ ;\ t' < 0]$ is different. For QPPS the quantum dissipation integral is still zero in these quadrants, while the same integral is larger than zero in the case of SPS. Hence, it can be concluded that the contribution of the quantum dissipation is larger in the case of a single phase slip compared to the case of when two phase slips tunnel into the loop simultaneously.

There is also another possible argument supporting the conclusion that QPPS can occur with a higher rate than SPS. The argument below does not involve the quantum dissipation

as an important factor, but involves the effective mass. The effective mass $m$ is strongly dependent Coulomb charging of the electrodes, *i.e.* the two segments of the center conductor (c.c.) of the resonator. It can be expected to be larger for SPS than for QPPS on the following grounds. The QPPS is an event in which two single phase slips are generated on both superconducting nanowires simultaneously (see Fig. 1). In such a case, the voltage generated by the phase slip on one wire would be opposite to the voltage on the other wire. These two locations of the electromotive force tend to move charges in the closed loop. As a result, they do not produce any significant charging of the electrodes. This is because the mean voltage produced by the phase slips is near zero. Therefore, the c.c. strips do not get charged in the course of the correlated tunneling of two phase slips. Therefore, the effective shunt capacitance becomes much smaller for QPPS, than it is for SPS. Small capacitance corresponds to a light phase particle, *i.e.* a much smaller effective mass for QPPS compared to SPS. (It should be reminded that the effective mass for phase slip events is defined by the Coulomb charging energy of the shunting capacitor.) Given the fact that, generally speaking, lighter particles tunnel with a higher rate compared to heavier particles, it can be concluded that the rate of macroscopic quantum tunneling should be much higher for QPPS than for SPS, because QPPS has a much smaller effective mass.

[1] A. Bezryadin, *Superconductivity in Nanowires: Fabrication and Quantum Transport* (Wiley-VCH, 69469 Weinheim, Germany, 2012).

[2] H. Kim, S. Jamali, and A. Rogachev, "Superconductor-insulator transition in long MoGe nanowires," Phys. Rev. Lett. **109**, 027002 (2012).

[3] R. Barends, J. Wenner, M. Lenander, Y. Chen, R. C. Bialczak, J. Kelly, E. Lucero, P. O'Malley, M. Mariantoni, D. Sank, H. Wang, T. C. White, Y. Yin, J. Zhao, A. N. Cleland, J. M. Martinis, and J. J. A. Baselmans, "Minimizing quasiparticle generation from stray infrared light in superconducting quantum circuits," Appl. Phys. Lett. **99**, 113507 (2011).

[4] T.O. Klaassen, J.H. Blok, J.N. Hovenier, G. Jakob, D. Rosenthal, and K.J. Wildeman, "Absorbing coatings and diffuse reflectors for the herschel platform sub-millimeter spectrometers HIFI and PACS," in *THZ 2002: IEEE Tenth International Conference on Terahertz Electronics Proceedings*, edited by J.M. Chamberlain, P. Harrison, R.E. Miles, A.G. Davies, E.H. Linfield, and S. Withington (2002) pp. 32–35.

[5] S. E. Korshunov, "Coherent and incoherent tunneling in a josephson junction with a"periodic" dissipation," JETP Lett. **45**, 434 (1987).

[6] F. Guinea and G. Schön, "Coherent charge oscillations in tunnel junctions," Europhys. Lett. **1**, 585 (1986).

[7] G. Schön and A. D. Zaikin, "Quantum coherent effects, phase transitions, and the dissipative dynamics of ultra small tunnel junctions," Phys. Rep. **198**, 237–412 (1990).
